# Supplementary material for: Towards a Neural Graphics Pipeline for Controllable Image Generation
Source: arXiv:2006.10569 source file (2021-02-22)
Supplement: Supplementary file 1 [file supp.tex]

\documentclass{article}

\usepackage{neurips_2020}

\usepackage[utf8]{inputenc} %
\usepackage[T1]{fontenc}    %
\usepackage{hyperref}       %
\usepackage{url}            %
\usepackage{booktabs}       %
\usepackage{amsfonts}       %
\usepackage{nicefrac}       %
\usepackage{microtype}      %

\usepackage{xspace}
\usepackage{enumerate}
\usepackage{graphicx}
\usepackage{sidecap}
\input{math_util}

\newcommand{\name}{Neural Graphics Pipeline\xspace}

\usepackage{color}
\definecolor{blue}{rgb}{0,0,1}
\definecolor{red}{rgb}{1,0,0}
\definecolor{green}{rgb}{0,.5,0}
\definecolor{orange}{rgb}{0.75, 0.4, 0}

\title{Supplementary: \name for Controllable Image Generation}

\begin{document}

\maketitle
\input{appendix}

\bibliographystyle{unsrt}
\bibliography{ref}

\end{document}
